# Supplementary material for: Topological Phononic Crystal on the Scale of Quasi-Ballistic Phonon Transport
Source: arXiv:2509.12528 source file (2025-09-16)
Supplement: Supplementary file 1 [file supplementary_material.pdf]

# Supporting information for "Topological Phononic Crystal in Scale of Quasi-Ballistic Phonon Transport"

Keita Funayama,<sup>\*,†</sup> Yuki Akura,<sup>‡</sup> Hiroya Tanaka,<sup>†</sup> and Jun Hirotsu<sup>‡</sup>

<sup>†</sup>*Toyota Central Research & Development Laboratories, Inc., Nagakute 480-1192, Japan*

<sup>‡</sup>*Department of Micro Engineering, Kyoto University, Kyoto 615-8540, Japan*

E-mail: funayama@mosk.tytlabs.co.jp

## Section 1: Estimation of a dominant phenomenon for thermal transport

We estimated the heat transfer in nanoscale silicon structures considering three representative mechanisms: thermal conduction (Figure S1(a)), natural convection (Figure S1(b)), and thermal radiation (Figure S1(c)). All three phenomena were assumed to be driven by the same temperature difference between the hot spot and the ambient environment,  $\Delta T = 10$  K. First, the heat transfer via thermal conduction through the fine beams,  $Q_{\text{cond}}$ , is expressed as  $Q_{\text{cond}} = \Delta T / (l / (k_{\text{eff}} w h_{\text{Si}}))$  W. For example, here,  $Q_{\text{cond}}$  is calculated by using parameters  $w = 0.2$ ,  $l = 4.0$ ,  $h_{\text{Si}} = 0.17 \mu\text{m}$ , and  $k_{\text{eff}}$  in  $\text{W}/(\text{m} \cdot \text{K})$ . In this case, the estimated heat transfer is  $Q_{\text{cond}} \approx 2.1 \times 10^{-6}$  W. Second, we consider thermal transfer from one site to the fine beam via air convection,  $Q_{\text{conv}}$ . The heat transfer depends on the surface area of the structure. The natural convection heat dissipation in air is expressed as  $Q_{\text{conv}} = \Delta T / (1 / (H \cdot S))$ , where  $H = 2000 \text{ W}/(\text{m}^2 \cdot \text{K})$  is the convective heat transfer coefficient and  $S$  is the surface area of the circular sublattice and fine beam. Using these values,  $Q_{\text{conv}} = 8.7 \times 10^{-7}$  W. Typically, the convective heat transfer coefficient  $H$  is  $1 \text{ to } 20 \text{ W}/(\text{m}^2 \cdot \text{K})$ . However, for nanoscale structures,  $H$  has been reported to increase to approximately  $2 \times 10^3$ .<sup>??</sup>

Finally, we calculated the thermal transfer via thermal radiation from the silicon structure,  $Q_{\text{radi}}$ . Similar to air convection, the amount of radiated heat increases with the surface area. Thus, the circular sublattice dominantly contributes to thermal radiation. Thermal radiation  $Q_{\text{radi}}$  is expressed as  $Q_{\text{radi}} = \sigma \epsilon S \Delta T (2T_0 + \Delta T) ((T_0 + \Delta T)^2 + T_0^2)$ , where  $\sigma = 5.67 \times 10^{-8} \text{ W}/(\text{m}^2 \cdot \text{K}^4)$  is the Stefan-Boltzmann constant,  $\epsilon = 0.7$  is the emissivity of single-crystal silicon, and  $T_0 = 293.15 \text{ K}$  ( $25^\circ\text{C}$ ) is the ambient temperature. Using these values, the heat transfer via thermal radiation is calculated as  $Q_{\text{radi}} = 1.77 \times 10^{-9}$  W. Emissivity  $\epsilon$  has been reported to change in nanoscale structures;<sup>??</sup> however,  $Q_{\text{radi}}$  does not increase significantly even if  $\epsilon$  approaches 1. As discussed above,  $Q_{\text{cond}}$  is at least one order of magnitude larger than  $Q_{\text{conv}}$  and  $Q_{\text{radi}}$ . Therefore, the dominant heat transfer pathway in

the fabricated structures is thermal conduction through the fine beams.

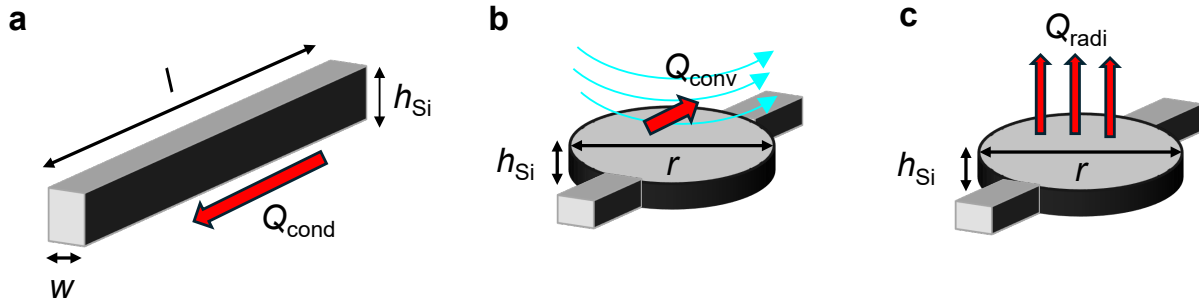

Figure S1: Schematics of thermal transfer via (a) thermal conduction through a fine beam, (b) air convection, and (c) thermal radiation.

## Section 2: Measurement of thickness of silicon device layer

We prepared silicon-on-insulator (SOI) substrates with silicon device layers of thicknesses 1.0, 0.17, and 0.07  $\mu\text{m}$ . The default thickness of the silicon device layer in the SOI was 1.0  $\mu\text{m}$ . The entire surface of the silicon device layers was etched using the Bosch process to obtain thicknesses of 0.17 and 0.07  $\mu\text{m}$ . Using these prepared SOI substrates, we fabricated nanoscale structures on the silicon device layer. After etching for device fabrication, the thickness of the silicon device layer was measured using a stylus profiler. Figure S2(a) and S2(b) show the thickness profiles for device layers reduced from 1.0  $\mu\text{m}$  to 0.17 and 0.07  $\mu\text{m}$ , respectively. The red lines in each inset indicate the positions where the profiling measurements were taken. Figures S2(a) and S2(b) show thickness profiles across the fine beams and circular sublattices, respectively. The color bars at the right edge of each profile provide a schematic representation of the SOI cross section based on the measured profiles. From Figure S2(a), the thickness of the silicon layer is observed to be  $th_{\text{Si}} \approx 0.17 \mu\text{m}$ . As shown in Figure S2(b), the thicknesses of the silicon layer and Au film are  $th_{\text{Si}} \approx 0.07 \mu\text{m}$  and  $th_{\text{Si}} \approx 0.56 \mu\text{m}$ , respectively. Therefore, we successfully prepared three nanoscale Si structures with different silicon device layer thicknesses.

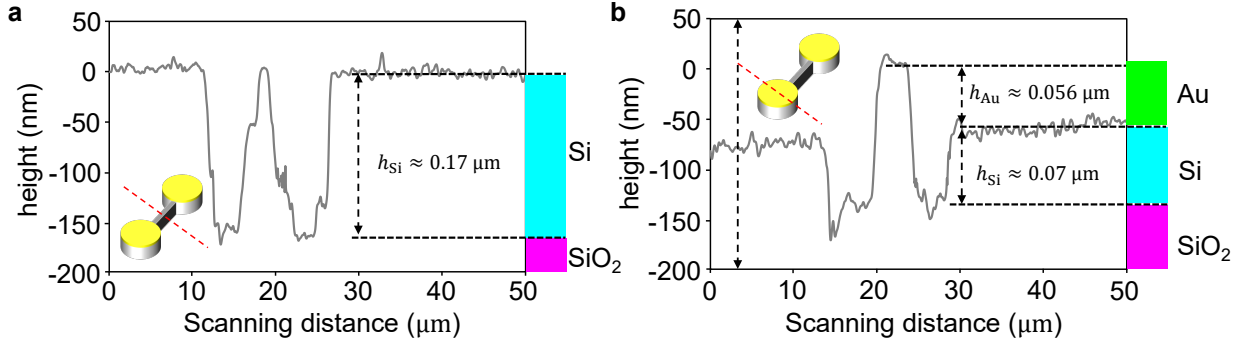

Figure S2: Thickness profiles of the silicon device layer for (a)  $h_{\text{Si}} \approx 0.17$  and (b)  $h_{\text{Si}} \approx 0.07 \mu\text{m}$ . The schematics in the inset of each profile represent the scanning line on the devices. The color bars at right edge of each profile are schematics of a cross section corresponding to the profiles.

### Section 3: Experimental and theoretical decay rate for topological interface states

Similar to Figure 4(a) in the main manuscript, Figures S3(a) and S3(b) show the decay rates of the nanoscale silicon structures for  $h_{\text{Si}} = 1.0$  and  $0.07 \mu\text{m}$ , respectively. Both results indicate that the experimental decay rates agree well with the theoretical decay rates for  $l_1 > 2 \mu\text{m}$ .

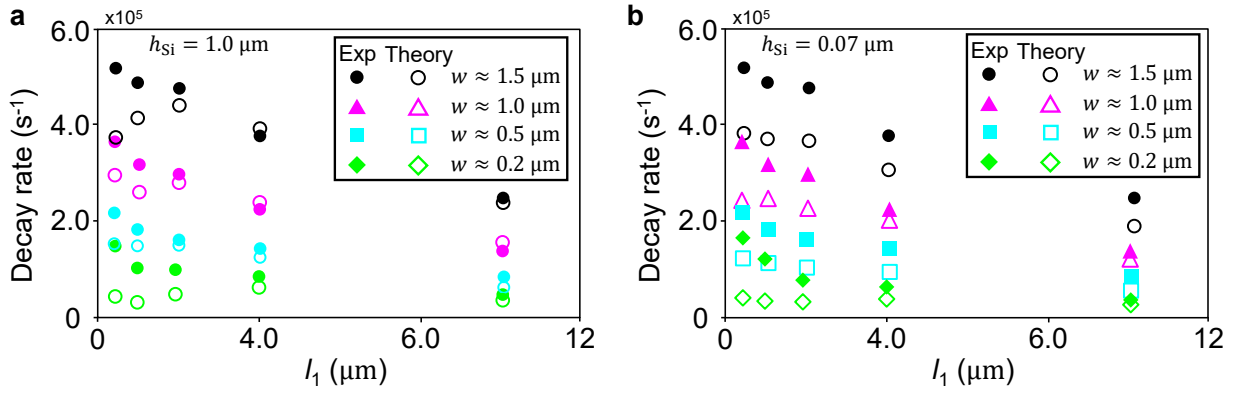

Figure S3: Experimental and theoretical decay rates as a function of fine beams with length  $l_1$  for the silicon nanoscale structures with (a)  $h_{\text{Si}} = 1.0$  and (b)  $h_{\text{Si}} = 0.07 \mu\text{m}$ . Each of the experimental decay rates were measured by heating only the  $n = 8$  site.
